# Supplementary material for: Quantum impurities in channel mixing baths
Source: arXiv:1509.01461 source file (2015-09-23)
Supplement: Supplementary file 1 [file SupplMater.pdf]

# Supplementary Materials for "Quantum impurities in channel mixing baths"

Jin-Guo Liu,[1] Da Wang,[1] and Qiang-Hua Wang[1,2,*]

[1]*National Laboratory of Solid State Microstructures & School of Physics, Nanjing University, Nanjing, 210093, China*

[2]*Collaborative Innovation Center of Advanced Microstructures, Nanjing University, Nanjing 210093, China*

In this Supplementary Materials, we provide technical details and numerical examples referred to in the main text. The numerical materials serve as justification of our mapping scheme proposed in the main text.

*Parametrization of $\epsilon_n(x)$ and $t_n(x)$*: For the purpose of NRG, we need a function $\epsilon_n(x)$ that becomes exponentially denser as $|x|$ increases. As in the usual logarithmic way, we define an auxiliary function

$$\varepsilon(x) = \min[(\omega_U - \omega_L)\Lambda^{2-|x|} + \omega_L, \omega_U] \; \mathrm{sign}(x), \quad \text{(S1)}$$

where $\omega_U$ and $\omega_L$ are upper and lower limits of $|\omega|$, representative of the bandwidth and energy gap, such that $\mathcal{D}(|\omega| > \omega_U) \equiv 0$ and $\mathcal{D}(|\omega| < \omega_L) \equiv 0$, and $\Lambda > 1$ is a scaling factor. We then define, for $|x| \geq 1$,

$$t_n(x) = \sqrt{\int_{\varepsilon[x+\mathrm{sign}(x)]}^{\varepsilon(x)} d\omega \; \rho_n(\omega) \; \mathrm{sign}(x)}, \quad \text{(S2)}$$

and we set $t_n(|x| < 1) \equiv 0$ for completeness. Combining Eq.(6) in the main text, which we reproduce here for convenience,

$$t_n(x)^2 |dx| = \rho_n[\epsilon_n(x)] \; |d\epsilon_n(x)|, \quad \text{(S3)}$$

we are also able to determine the fictitious energy level $\epsilon_n(x)$, starting from $|x| = 1$ where $\epsilon_n(\pm 1) = \pm\omega_U$. It can be shown that the resulting $\epsilon_n(x)$ lies in between $\varepsilon(x)$ and $\varepsilon[x + \mathrm{sign}(x)]$, so that $\epsilon_n(x)$ inherits the sign and scaling behavior of $\varepsilon(x)$, as would have been desired.

*Numerical examples*: We discretize the s-wave superconducting bath as discussed in the main text. We set $\pi\Gamma = 0.5$ and $\Delta = 0.1$, and we take $\omega_U = \sqrt{1 + \Delta^2}$ and $\omega_L = \Delta$ as the cutoff energies due to the pairing gap $\Delta$. To check the precision of this mapping, we use the resulting discretized model to recalculate

$$\mathcal{D}_{\alpha\beta}(\omega) = \sum_{n,j\neq 0} V_{\alpha n}(x_j)\delta[\omega - \epsilon_n(x_j)]V^\dagger_{n\beta}(x_j), \quad \text{(S4)}$$

where $V_{\alpha n}(x) = t_n(x)\langle\alpha|n, x\rangle$ and $x_j = (|j| + \eta)\mathrm{sign}(j)$, as defined in the main text. We average the result over 50 twisting factors $\eta$ uniformly distributed in $(0, 1]$. The resulting components in $\mathcal{D}(\omega) = d_0(\omega)\sigma_0 + d_x\sigma_x(\omega)$ are compared to the analytical ones in Fig.S1 (left panel). We see excellent agreement in the low energy window. The deviation at the band edges is an artifact due to the larger smearing factor we used for larger energies.

We proceed to perform the mapping to the Wilson chain, and we use this chain to calculate $\mathcal{D}(\omega)$ again as follows. We define a recursive Green's function, for decreasing $k$,

$$G_k^{-1}(z) = z\mathbf{1} - E_k - T_k G_{k+1}(z) T_k^\dagger, \quad \text{(S5)}$$

where $z$ is a complex frequency, $\mathbf{1}$ is an identity matrix, and $E_k$ and $T_k$ are matrices defined and calculated as described in the main text for the Wilson chain. The initial condition in the recursion is

$$G_K^{-1}(z) = z\mathbf{1} - E_K, \quad \text{(S6)}$$

where $K$ is the length of the chain. Then the self-energy correction to the impurity is given by

$$\Sigma(z) = T_0 G_1(z) T_0^\dagger, \quad \text{(S7)}$$

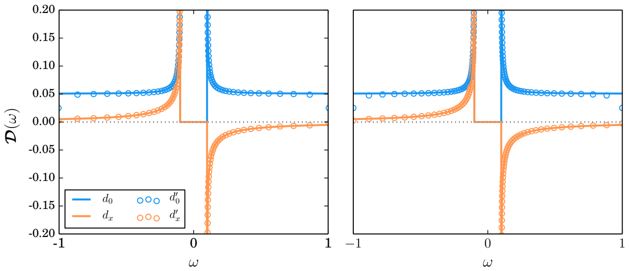


FIG. S1. Comparison of the analytical $d_0(\omega)$ and $d_x(\omega)$ (solid lines) and numerical results $d'_0(\omega)$ and $d'_x(\omega)$ (symbols) obtained from the discrete bath (left panel) the open Wilson chain (right panel). The scaling parameter $\Lambda = 3$ and the number of block-Lanczos iterations is $J = 25$. The result is averaged over 50 twisting factors $\eta$ uniformly distributed in $(0, 1]$.

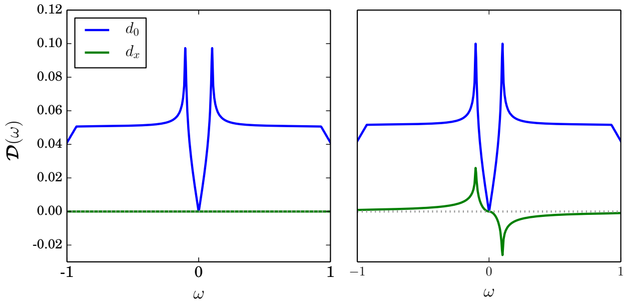


FIG. S2. Components of the hybridization function for an Anderson impurity coupled to a $d$-wave superconductor for $t_2/t_0 = 0$ (left panel) and $t_2/t_0 = 0.1$ (right panel). In both cases $t_0$ is fixed by $\pi\Gamma = 0.5$.

which is used to recalculate $\mathcal{D}(\omega)$ by

$$\mathcal{D}(\omega) = i[\Sigma(\omega + i0^+) - \Sigma(\omega - i0^+)]/2\pi. \tag{S8}$$

We present the resulting $d_{0,x}(\omega)$, averaged over $\eta$ as above, and compare to the analytical results in Fig.S1 (right panel). The agreement within each panel and the consistency between the two panels reveal the nice accuracy and consistency of our two-stage mapping scheme.

For the $d$-wave superconducting bath with a gap amplitude $\Delta = 0.1$ and with $\pi\Gamma = 0.5$ (which determines $t_0$) discussed in the main text, we set $\omega_U = \sqrt{1+\Delta^2}$ and $\omega_L = 0$. After the mapping to the Wilson chain, we recalculate $\mathcal{D}(\omega)$ using the recursive Green's function method described above. The components of the resulting $\mathcal{D}(\omega)$ are shown in Fig.S2 for $t_2/t_0 = 0$ (left panel) and $t_2/t_0 = 0.1$ (right panel). The result is indistinguishable to the starting analytical $\mathcal{D}(\omega)$ in the main text (not shown), except for the artifact at the band edges as mentioned above. Fig.S1 and Fig.S2 serve as a solid justification of our mapping scheme.

For technical details, we have uploaded the python program and technical manual to the Github, https://github.com/GiggleLiu/nrg_mapping Numerical tests for 2- and 4-channel hybridization functions, with channel mixing, are available in this web site.

* qhwang@nju.edu.cn
